# Supplementary material for: Stein Variational Probabilistic Roadmaps
Source: arXiv:2111.02972 source file (2022-05-20)
Supplement: Supplementary file 1 [file appendix.tex]

\section*{APPENDIX}
\label{sec:appendix}

% Appendixes should appear before the acknowledgment.
